# Supplementary material for: Multi-Modal Multi-Agent Optimization for LIMMS, A Modular Robotics Approach to Delivery Automation
Source: arXiv:2208.00495 source file (2022-07-31)
Supplement: Supplementary file 1 [file SA1_appendix.tex]

\section{Appendix}
\label{sec:appendix}

Equation.
